# Supplementary material for: Advancing Earth Observation: A Survey on AI-Powered Image Processing in Satellites
Source: arXiv:2501.12030 source file (2025-01-21)
Supplement: Supplementary file 1 [file Appendix.tex]

% \newpage
% \section{Appendix}
% The larger results tables have been made available through a github.io page which can be viewed \href{https://aidanduggancit.github.io/SGAI/SGAI.html}{here}

% \begin{table}[h]
%     \centering
%     \includegraphics[width=\textwidth]{Figures/Acc_Energy_Table.jpg}
%     \caption{All Models - Accuracy / Energy}
%     \label{table:Acc_Energy_Table}
% \end{table}

% \begin{table}[h]
%     \centering
%     \includegraphics[width=\textwidth]{Figures/Latency_Energy_Table.jpg}
%     \caption{All Models - Latency / Energy}
%     \label{table:Latency_Energy_Table}
% \end{table}
